# Supplementary material for: RETHINED: A New Benchmark and Baseline for Real-Time High-Resolution Image Inpainting On Edge Devices
Source: arXiv:2503.14757 source file (2025-03-18)
Supplement: Supplementary file 1 [file X_suppl.tex]

%\clearpage
%\setcounter{page}{1}
%\maketitlesupplementary

\subsection{Training}\label{sec:training}
We train our inpainting model using a loss consisting of perceptual, error-based (both in space and frequency values), and adversarial components. Indeed, our loss consists of four terms. First, an L$^2$ error-based loss comparing the inpainted coarse image $\hat{\mathbf{x}}_{\text{coarse}}$ with the LR image ${\mathbf{x}}_{\text{LR}}$. Second, an error term based on the difference in Fourier frequencies (obtained from the Fast Fourier Convolutions operator~\cite{chi2020fast}) of the inpainted image $\hat{\mathbf{x}}_\text{LR}$ and the LR input image ${\mathbf{x}}_{\text{LR}}$. In particular, we use the Focal Frequency
loss that favors similarity in the spectral domain and encourages details and high frequencies \cite{jiang2021focal}. %\cite{jiang2021focal,suvorov2022resolution,sanchez2022photorealistic}. 
Third, a 
perceptual term based on a high receptive field network \cite{zhang2018unreasonable,suvorov2022resolution} comparing again the inpainted image  $\hat{\mathbf{x}}_\text{LR}$ with the input coarse image ${\mathbf{x}}_{\text{LR}}$ in order to force structure.
%This set of deep and non-deep perceptual losses 
Finally, following the well-known adversarial training, we use a discriminator based on patch-GAN architecture~\cite{isola2017image}.

%\vspace*{20mm}
%\twocolumn[{%
%\renewcommand\twocolumn[1][]{#1}%
%\maketitle
%\begin{center}
    \centering
    \captionsetup{type=figure}
    \includegraphics[width=0.5\textwidth]{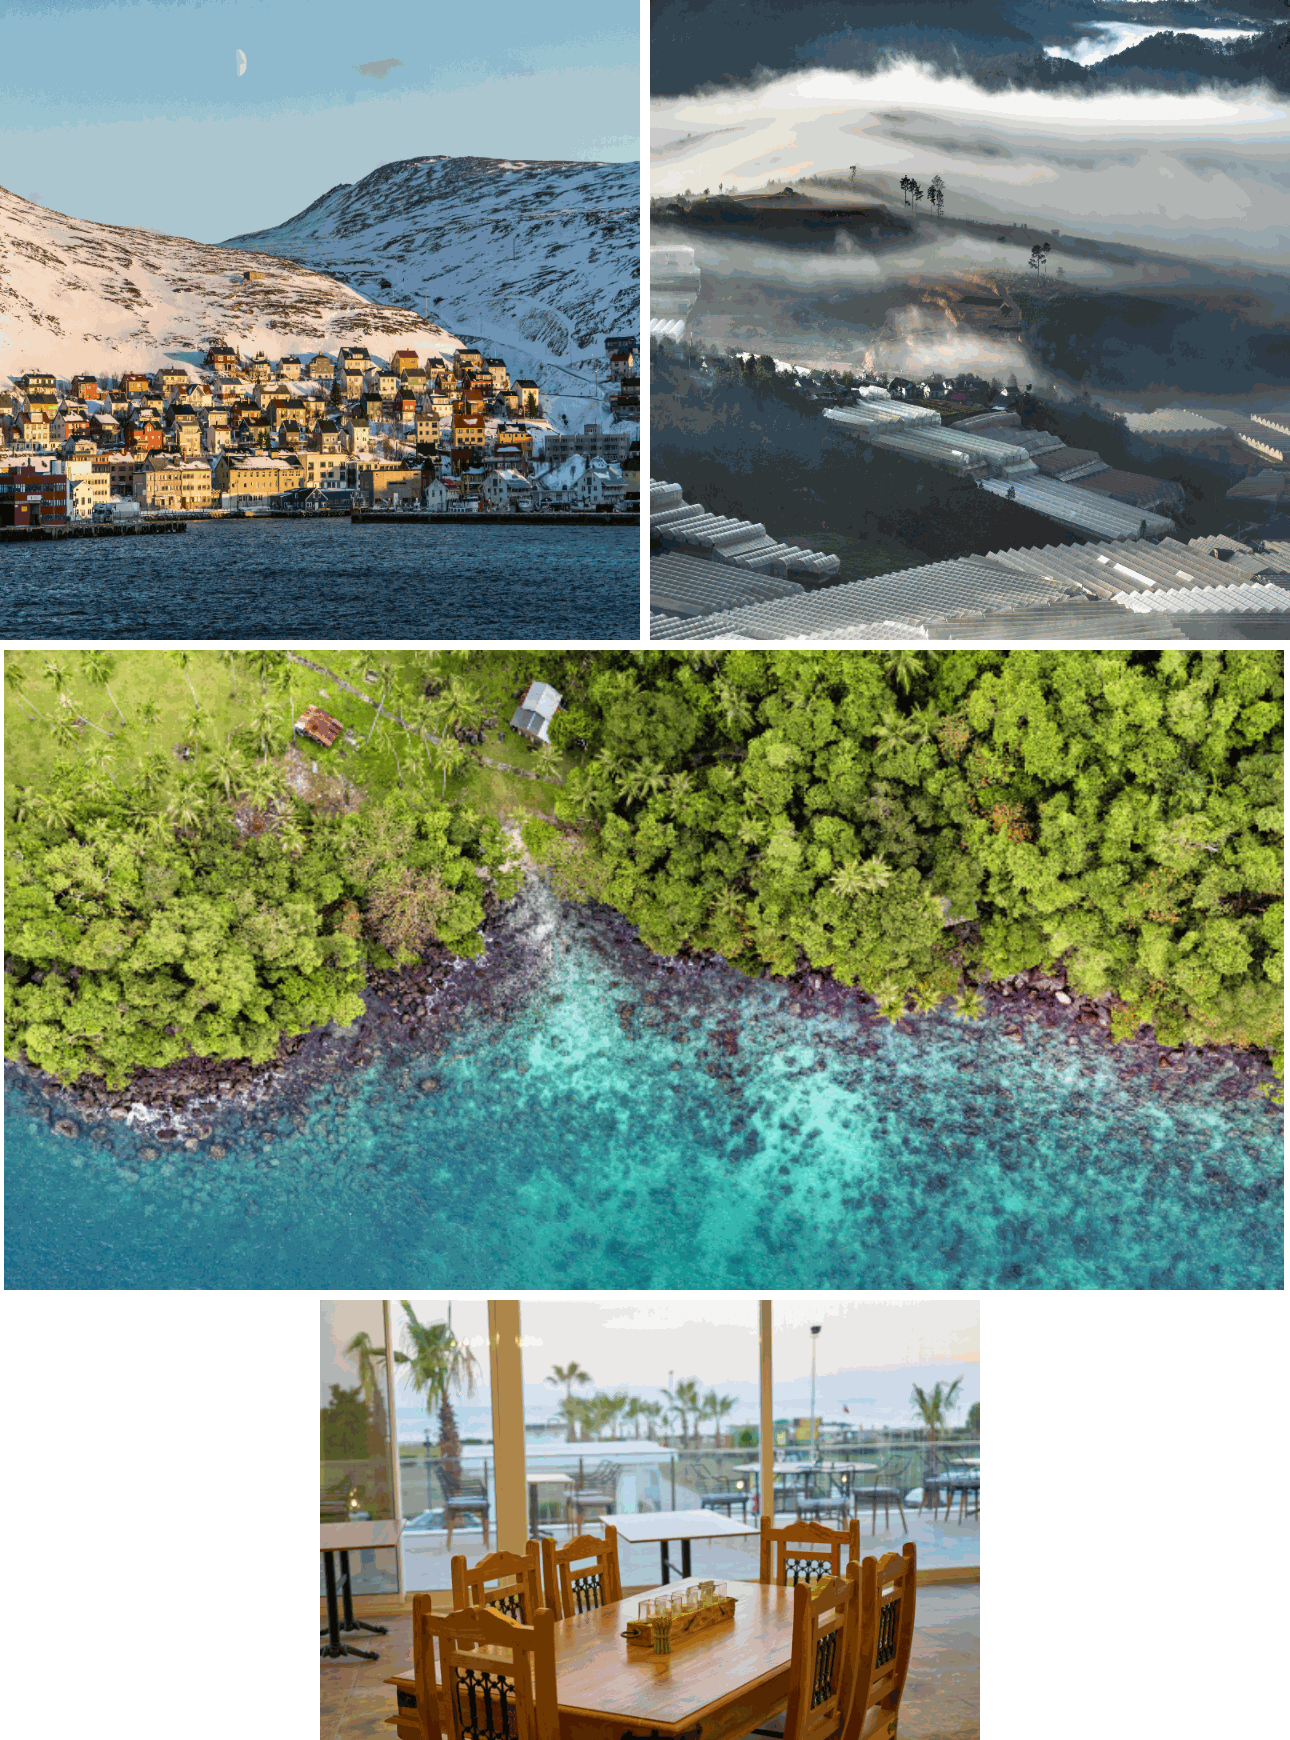}
    \caption{\textbf{High Resolution Samples from DF8k-Inpainting Dataset.}}
%\end{center}%
%}]

%\twocolumn[{%
%\renewcommand\twocolumn[1][]{#1}%
%\maketitle
\begin{center}
    \centering
    \captionsetup{type=figure}
    \includegraphics[width=0.5\textwidth]{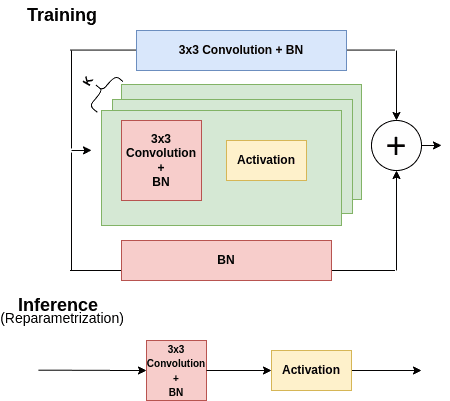}
    \caption{\textbf{Reparametrization tecnique used in inference to improve latency speed.}}
    \label{fig:reparametrization}
\end{center}%
%}
%]

\section{Efficient Img2Col}
\label{sec:efficientImg2Col}

\begin{algorithm}[h]
\SetAlgoLined
    \PyCode{weights = torch.eye (kernelSize, dtype=torch.float)}
    \\
    \\
    \PyCode{weights=weights.reshape((kernelSize ** 2,
             1, kernelSize, kernelSize)}
    \\
    \PyCode{weights = weights.repeat(3, 1, 1, 1)}
    \\
    \\
    \PyCode{patches = \text{F.Conv2d}(
            inputImage,
            weights,
            bias=None,
            stride=kernelSize,
            padding=0,
            dilation=1,
            groups=3,
        )}
    \\
    \PyCode{return patches}
\caption{PyTorch pseudocode for img2col}
\label{algo:img2col}
\end{algorithm}

In orde to efficiently split the the image into patches, several approaches exist. Most methods follow standard implementation \cite{dosovitskiy2020image}, which make use of use operations such us \texttt{permute} or \texttt{view} which hurt performance on edge devices. In order to avoid memory bound operation such as the previously described, we implemented the \texttt{Img2Col} operation via a 2D convolution. To do so, we generate the weights $\mathbf{w} \in \mathbb{R}^{{P} \times {P}}$ where:

\begin{equation}
\mathbf{w}(i,j) = 
\left\{
    \begin{array}{ll}
        1, & \text{if } i = j \\
        0, & \text{otherwise}
    \end{array}
\right.
\end{equation}
In order to match the input channel, we duplicate the channels to match input dimension. A more detailed pseudo-code can be found in Algorithm \ref{algo:img2col}.

% \section{Coarse Model}
% \label{sec:efficientImg2Col}

% The coarse model is based on a Unet network, composed by an encoder and a decoder. The encoder is a mobileOne \cite{vasu2023mobileone} backbone  with 5 blocks. The decoder is a composed by 4 blocks of convolution and bicubic Upsampling. At inference, the encoder is parametrized to improve latency performance, as displayed in \ref{fig:reparametrization}.

% \section{Super High-resolution Inpainting Examples}
% \twocolumn[{%
% \renewcommand\twocolumn[1][]{#1}%
% \maketitle
% \begin{center}
%     \centering
% \begin{tikzpicture}[spy using outlines={thick,red,rectangle,magnification=5,size=5cm,connect spies}]
%     \node[rectangle,draw,inner sep=0pt] (image) at (0,0){\includegraphics[width=\textwidth]{teaser_fig/inpainted_high_res_2048_51095511725_7c9a8a4640_4k_0_0.png}};
%     \spy[spy connection path={
%     %\draw[densely dashed] (tikzspyinnode.north west) -- (tikzspyonnode.north west);
%     %\draw[densely dashed] (tikzspyinnode.south west) -- (tikzspyonnode.south west);
%     %\draw[densely dashed] (tikzspyinnode.north east) -- (tikzspyonnode.north east);
%     %\draw[densely dashed] (tikzspyinnode.south east) -- (tikzspyonnode.south east);
% }]on (-2.6,1.0) in node at (6.25,-4.1);
% \end{tikzpicture}&
%     \captionof{figure}{Test caption \gt{(I assume this entire figure will be redone with a better example and fancier scatterplot?)}}
% \end{center}%
% }]
